# Supplementary material for: Do I Belong? Modeling Sense of Virtual Community Among Linux Kernel Contributors
Source: arXiv:2301.06437 source file (2023-02-23)
Supplement: Supplementary file 1 [file appendix.tex]

\appendix

\section{Demographics}
\begin{table}[htb]
\centering
\caption{Demographics of the Linux Kernel respondents (n=217)}
\label{tab:demographics}

\begin{tabular}{p{4cm}p{2cm}p{1cm}}
\toprule
Attribute & N & Percentage\\
\midrule
\multicolumn{3}{c}{Gender}\\
\midrule
Man & 190 & 87.6\%\\
Woman & 21 & 9.7\%\\
Non-binary & 5 & 2.3\%\\
Prefer to self describe & 1 & 0.4\%\\
\midrule
\multicolumn{3}{c}{Country of Residence}\\
\midrule
USA & 61 & 28.1\%\\
Germany & 27 & 12.4\%\\
UK & 20 & 9.2\%\\
India & 13 & 6.0\%\\
Italy & 9 & 4.1\%\\
China & 8 & 3.7\%\\
France & 7 & 3.2\%\\
Brazil & 6 & 2.8\%\\
Romania & 6 & 2.8\%\\
Canada & 5 & 2.3\%\\
Finland & 5 & 2.3\%\\
Spain & 5 & 2.3\%\\
Sweden & 5 & 2.3\%\\
Czech Republic & 4 & 1.8\%\\
Israel & 4 & 1.8\%\\
Japan & 4 & 1.8\%\\
Australia & 3 & 1.4\%\\
Netherlands & 3 & 1.4\%\\
Poland & 3 & 1.4\%\\
Pakistan & 2 & 0.9\%\\
Switzerland & 2 & 0.9\%\\
Taiwan & 2 & 0.9\%\\
Other countries & 13 & 6.0\%\\
\midrule
\multicolumn{3}{c}{Starting year at the Linux Kernel}\\
\midrule
2000 or earlier & 27 & 12.4\%\\
Between 2001 and 2010 & 74 & 34.1\%\\
Between 2011 and 2021 & 116 & 53.5\%\\
\midrule
\multicolumn{3}{c}{Current Compensation for the Linux Kernel contributions}\\
\midrule
Paid & 142 & 65.4\%\\
Unpaid (volunteer) & 75 & 34.6\%\\
\bottomrule

\end{tabular}
\end{table}

\section{Survey Instrument}
\label{sec:appendix}

This sample study was conducted via an online survey implemented with LimeSurvey. The full survey instrument is listed below. Items prefixed with a (*) were dropped due to poor loading onto their constructs (see Section \ref{xxx} for details).

\textsc{\textbf{Motivations}}: How important are these reasons for you to contribute to the Linux Kernel? (5-points Likert - Not Important, Slightly Important, Moderately Important, Important, Very Important)
\begin{itemize}
    \item I have fun contributing (Fun)
    \item I feel personal obligation because I use, want to improve the quality of the project I'm working on, or believe source code should be open (Ideology/Reciprocity)
    \item I like the collaborative environment, deeply enjoy helping others, want to share knowledge, want to participate in the scene, or like to work with this development team (Kinship/Altruism)
\end{itemize}

\textsc{\textbf{Sense of Virtual Community}}: How do you feel about the subsystem(s) of the Linux development community you contribute to? (5-points Likert - Strongly Disagree, Disagree, Neither Agree nor Disagree, Agree, Strongly Agree)
\begin{itemize}
    \item svc1. I don't feel at home in the group
    \item svc2. I feel that I belong to the group
    \item svc3. If I have a problem, I know members in the group who I can ask for help
    \item svc4. I want to contribute more but I do not feel valued
    \item svc5. A majority of developers in the group know me
    \item svc6. The majority of the developers and I want the same thing (*)
\end{itemize}

\textsc{\textbf{English Confidence}}: How confident are you in your ability to read, write and speak in English when performing the following activities? (please choose the appropriate response for each item) (5-points Likert - Uncomfortable, Not confident (can manage, but difficult), Average, Confident, Very Confident (fluent))
\begin{itemize}
    \item eng1. Participating in a non-technical discussion on the email list
    \item eng2. Performing Reviews
    \item eng3. Speaking with others (face to face)
    \item eng4. Participating in technical discussions on the email list
\end{itemize}

\textsc{\textbf{Gender}}: My gender identity is:
\begin{itemize}
    \item Woman
    \item Man
    \item Non-Binary
    \item Prefer to Self-Describe
    \item Prefer not to Say
\end{itemize}

\textsc{\textbf{Country:}} In which country do you currently reside?
\begin{itemize}
    \item (drop-down list with countries)
\end{itemize}

\textsc{\textbf{Compensation:}}\\
Have you ever been paid to contribute to the Linux Kernel?
\begin{itemize}
    \item Yes
    \item No
\end{itemize}
When have you been paid to contribute to the Linux Kernel? (displayed if the answer for previous question is Yes)
\begin{itemize}
    \item I’ve only been paid to make my first contribution (currently unpaid)
    \item I’ve been paid to make some past contributions but I’m not anymore (currently unpaid)
    \item I’m currently being paid to make all (or part of) my contributions
\end{itemize}

\textsc{\textbf{Tenure:}} When did you first contribute to the Linux Kernel (year)?
